# Supplementary material for: Electronic Structures and Optical Properties of Partially and Fully Fluorinated Graphene
Source: arXiv:1408.4717 source file (2015-02-24)
Supplement: Supplementary file 1 [file CF_v9_Supplement.pdf]

# Supplemental Material to
# Electronic Structures and Optical Properties of Partially and Fully Fluorinated Graphene

Shengjun Yuan,[1,*] Malte Rösner,[2,3] Alexander Schulz,[2,3] Tim O. Wehling,[2,3] and Mikhail I. Katsnelson[1]
[1] *Institute for Molecules and Materials, Radboud University Nijmegen, Heyendaalseweg 135, 6525AJ Nijmegen, The Netherlands*
[2] *Institut für Theoretische Physik, Universität Bremen, Otto-Hahn-Allee 1, 28359 Bremen, Germany*
[3] *Bremen Center for Computational Materials Science, Universität Bremen, Am Fallturm 1a, 28359 Bremen, Germany*

## TIGHT-BINDING MODEL

To be able to treat general disorder configurations, we construct a tight-binding (TB) model which is capable of describing pristine, fully and partially fluorinated graphene. To this end, we use a multi-orbital tight-binding Hamiltonian

$$\mathbf{H} = \sum_{\alpha i} \varepsilon^i_\alpha n_{i,\alpha} + \sum_{\alpha\beta<ij>} t^{ij}_{\alpha\beta} c^\dagger_{i,\alpha} c_{j,\beta}, \qquad (1)$$

where $i, j$ are site indices, $\alpha$ and $\beta$ label the orbital basis $\{\text{carbon} : s, p_x, p_y, p_z \ \text{fluorine} : p_x, p_y, p_z\}$, $< ij >$ indicates summation over nearest neighbours and $t^{ij}_{\alpha\beta}$ are hopping matrix elements. The exact definition of $t^{ij}_{\alpha\beta}$ and the involved direction cosines can be found in Table I and Table II. The two-center integrals involved in the definition of the hopping matrix elements are determined by fitting the TB band structures to *ab initio* data, which has been done for pristine and fully fluorinated graphene separately.

Since it is known, that the bandgap of fluorographene is underestimated in density functional theory (DFT) calculations, we use the $G_0W_0$ method to include non-local screened exchange self-energy corrections to the DFT eigenenergies for both, fluorographene and pristine graphene[1]. We use the PAW method as implemented in the VASP code[2] to obtain converged GGA (PBE) DFT calculations as starting points for the $G_0W_0$ calculations. In all cases a $8 \times 8 \times 1$ k-mesh and an energy cut off of 400 eV. is used. For pristine graphene we use a lattice constant of $a_0 = 2.47$ Å. The geometry of fluorographene (chair configuration, see Fig. 1) has been optimized, which yields a lattice constant of $a_0 = 2.62$ Å, an out-of-plane displacement of $\Delta_z = \pm 0.21$ Å for each carbon atom and a fluorine-carbon-distance of $c = 1.38$ Å. The $G_0W_0$ calculations included Bloch states up to an energy of 120 eV in all calculations. The resulting $G_0W_0$ quasiparticle energies for graphene and fluorographene are used to fit the nearest neighbor TB model from Eq. (1). The resulting parameters for each system can be found in Table III and the corresponding band structures and density of states (DOS) can be seen in Fig. 2 and Fig. 3, respectively. To plot the $G_0W_0$ band structure we interpolate the renormalized quasiparticle energies using Wannier functions.

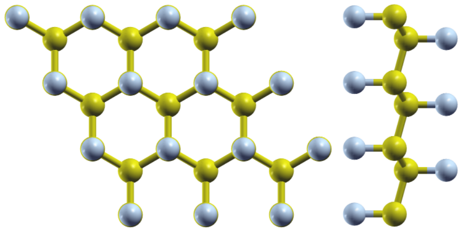

Figure 1. Fluorographene in chair configuration (yellow: carbon, gray: fluorine)

| | |
|---|---|
| $t_{ss}$ | $V_{ss\sigma}$ |
| $t_{sp_x}$ | $lV_{sp\sigma}$ |
| $t_{p_xp_x}$ | $l^2V_{pp\sigma} + (1-l^2)V_{pp\pi}$ |
| $t_{p_xp_y}$ | $lm(V_{pp\sigma} - V_{pp\pi})$ |

Table I. Definition of Slater-Koster parameters. Not listed elements can be obtained by permutation of the indices and nearest neighbor direction cosines $(l, m, n)$.

It is obvious, that the simple nearest neighbor TB models are not able to describe every single detail of the original band structures. Nevertheless, the most important features, like the linear dispersion around the Dirac point in graphene or the states around the conduction and valence band edges in fluorographene are reproduced.

In the case of fluorographene we end up with a band gap of 6.3 eV, which is about 0.7 eV smaller than recently published $G_0W_0$ calculations[3] for a free standing layer. Here, adjacent layers are separated by about 10 Å which is one third of the distance used in Ref. [3]. Therefore, screening effects due to the Coulomb interaction ($W_0$ in $G_0W_0$) from neighboring slabs are present, which models an effective dielectric environment and which lowers the band gap. This effect mimics the influence of a dielectric substrate with a static dielectric constant of 1.8 in the long wavelength limit.

To model partially fluorinated graphene, we use a supercell in which randomly (or ordered) fluorine atoms are introduced. Thereby, three different carbon-carbon hopping combinations arise: 1.) nearest neighbor hopping between pristine carbon atoms (graphene like hopping,

| | graphene | | | fluorographene | | | $CF_x$ | | |
|---|---|---|---|---|---|---|---|---|---|
| $\boldsymbol{\delta}_i$ | $l_i$ | $m_i$ | $n_i$ | $l_i$ | $m_i$ | $n_i$ | $l_i$ | $m_i$ | $n_i$ |
| $\boldsymbol{\delta}_1$ | 0 | 1 | 0 | 0 | +0.964 | -0.265 | 0 | +0.991 | -0.136 |
| $\boldsymbol{\delta}_2$ | $-\sqrt{3}/2$ | $-1/2$ | 0 | −0.835 | −0.482 | -0.265 | −0.856 | −0.495 | -0.136 |
| $\boldsymbol{\delta}_3$ | $+\sqrt{3}/2$ | $-1/2$ | 0 | +0.835 | −0.482 | -0.265 | +0.856 | −0.495 | -0.136 |
| $\boldsymbol{\delta}_F$ | 0 | 0 | 0 | 0 | 0 | 1 | 0 | 0 | 1 |

Table II. Direction cosines. Here $\boldsymbol{\delta}_F$ denotes the vector of the adjacent upper F atom of the central C atom.

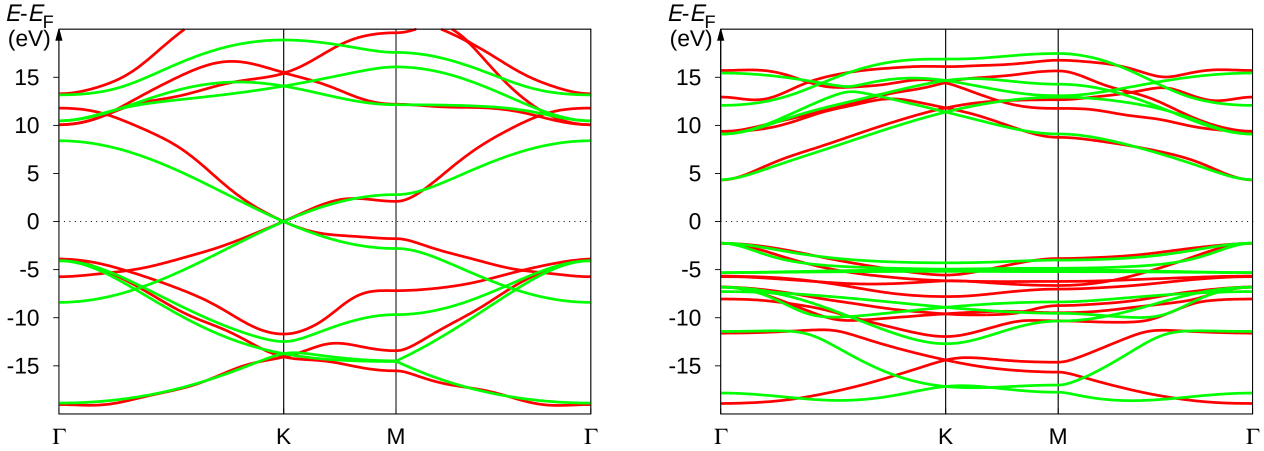


Figure 2. Wannier interpolated $G_0W_0$ (red) and TB (green) band structures of graphene (**left**) and fluorographene (**right**). The dotted line at $E = 0\,\mathrm{eV}$ illustrates the common reference energy.

denoted by GR in Tab. III), 2.) hopping between two fluorinated carbon atoms (fluorographene like hopping, denoted by FGR) and 3.) hopping between a pristine and a fluorinated carbon atom. Thus, the local environment has to be considered to choose the correct hoppings and onsite energies for partially fluorinated graphene. In the case of a hopping between two unfluorinated carbon atoms we use the GR labelled column of Tab. III. In the second case of a hoping between two fluorinated carbon atoms we use the FGR labelled column and in the third case, which is about a hopping between an unfluorinated and a fluorinated carbon atom we just take the arithmetic mean value of the corresponding values from the GR and FGR columns together with the $CF_x$ direction cosines from Tab. II. The carbon onsite energies for a partially fluorinated system are chosen corresponding to the fact, whether the carbon atom is fluorinated or not. Hence, special care must be taken to choose the correct onsite energies or hoppings in the case of partially fluorinated graphene.

Furthermore, since a common reference energy of pristine and fully fluorinated graphene is a priori not known, special care must be taken in using the TB onsite energies in the case of partially fluorinated graphene. We determine this common reference energy by matching the *ab initio* local DOS (LDOS) of a single fluorine impurity (and its surrounding) with the corresponding LDOS of the TB model. To this end, we use a relaxed graphene supercell including 16 carbon atoms with a single fluorine impurity. As in the previous cases we perform a $G_0W_0$ calculation including Bloch states up to an energy of 120 eV. The *ab initio* LDOS predicts a midgap state around the Fermi energy with coinciding maxima of the surrounding LDOS. We define the Fermi energy of pristine graphene to be at 0 eV, i.e. all single particle energies are given relative to this Fermi level. Then, all on-site energies in the TB description of fluorographene are adjusted until the impurity induced maxima of the LDOS obtained from the TB model of the supercell containing the fluorine impurity on graphene match the $G_0W_0$ results, as can be seen from Fig. 4 and Fig. 3 c). This offset is included in the parameters given in Tab. III, yielding correctly aligned on-site energies energies. Thereby, the Fermi energies in all models are set to 0 eV. The corresponding total DOS of the TB model compared to the original $G_0W_0$ DOS can be seen in the Fig. 3 c). Next to the valence band, the impurity state is reproduced in good approximation.

## OPTICAL PROPERTIES

The real part of optical conductivity is calculated by using the Kubo formula in the form [4, 5]

$$\sigma_{\alpha\beta}(\omega) = \lim_{\varepsilon\to 0^+} \frac{e^{-\beta\omega}-1}{\omega\Omega} \int_0^\infty e^{-\varepsilon t} \sin\omega t \times 2\mathrm{Im}\,\langle\varphi| f(\mathbf{H})\, J_\alpha(t)\, [1 - f(\mathbf{H})]\, J_\beta|\varphi\rangle\, dt, \quad (2)$$

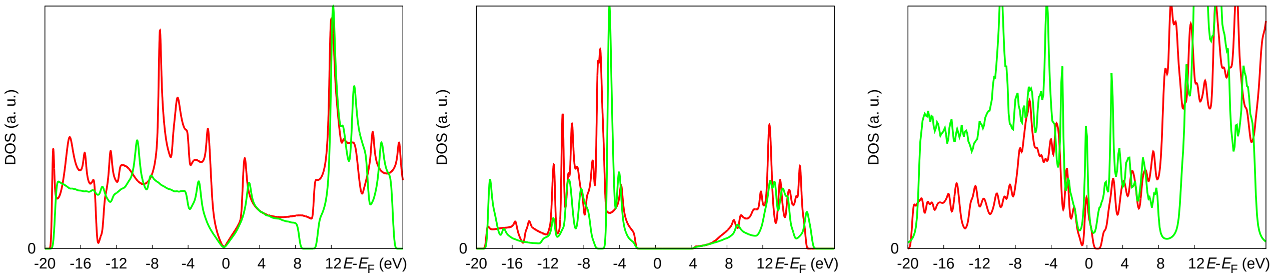


(a) graphene (b) fluorographene (c) fluorine impurity in a supercell of 16 carbon atoms

Figure 3. Total DOS of the TB models (green) and the *ab initio* calculations (red). In the case of graphene and fluorographene the *ab initio* DOS is calculated using the Wannier constructions shown in Fig. 2, whereas the *ab initio* DOS of the supercell shows the original $G_0W_0$ data.

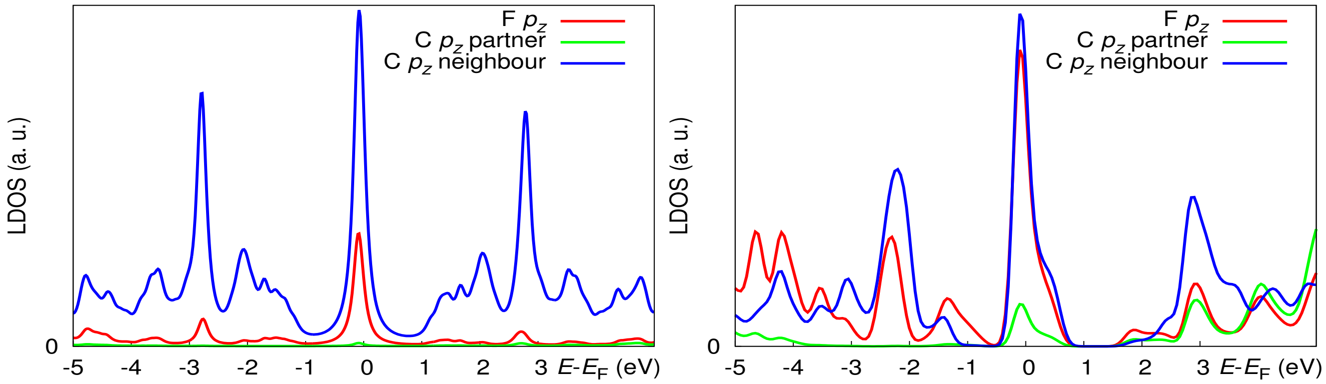


Figure 4. **Left:** TB $p_z$ LDOS of a fluorine impurity in a supercell of 16 carbon atoms together with the corresponding LDOS of the carbon bonding partner and its nearest neighbor carbon atom using the parameters of Table III. **Right:** Corresponding $G_0W_0$ results

| | GR | FGR |
|---|---|---|
| $\varepsilon_s$ | $-2.85$ | $-5.54$ |
| $\varepsilon_{p_{xy}}$ | $+3.20$ | $+2.31$ |
| $\varepsilon_{p_z}$ | $+0.00$ | $+4.92$ |
| $V_{ss\sigma}$ | $-5.34$ | $-3.65$ |
| $V_{sp\sigma}$ | $+6.40$ | $+7.20$ |
| $V_{pp\sigma}$ | $+7.65$ | $+7.65$ |
| $V_{p_{xy}p_z\sigma}$ | $+0.00$ | $+2.20$ |
| $V_{p_{xy}p_{xy}\pi}$ | $-2.80$ | $-2.64$ |
| $V_{p_{xy}p_z\pi}$ | $+0.00$ | $-2.80$ |
| $V_{p_zp_z\pi}$ | $-2.80$ | $-1.87$ |
| $\varepsilon^F_{p_{xy}}$ | | $-4.94$ |
| $\varepsilon^F_{p_z}$ | | $-1.69$ |
| $V^{C-F}_{sp\sigma}$ | | $+1.06$ |
| $V^{C-F}_{pp\sigma}$ | | $+9.85$ |
| $V^{C-F}_{pp\pi}$ | | $-2.25$ |

Table III. Two-center integrals involved in the definition of the Slater-Koster parameters for graphene (GR) and fluorographene (FGR). The upper panel shows the carbon onsite energies as well as the carbon-carbon hopings, while the lower panel shows the the fluor onsite energies and the corresponding carbon-fluor hoppings. All values are given in eV.

where $\beta = 1/k_BT$ is the inverse temperature, $\Omega$ is the sample area, $f(\mathbf{H}) = 1/\left[e^{\beta(\mathbf{H}-\mu)}+1\right]$ is the Fermi-Dirac distribution operator, $|\varphi\rangle$ is a random superposition of all the basis states in the real space, i.e., $|\varphi\rangle = \sum_i a_i c_i^\dagger |0\rangle$[5, 6] where $a_i$ are random complex numbers normalized as $\sum_i |a_i|^2 = 1$, and $|0\rangle$ is the electron vacuum state. The time-dependent current operator in the $\alpha$ $(= x,y$ or $z)$ direction is $J_\alpha(t) = e^{i\mathbf{H}t} J_\alpha e^{-i\mathbf{H}t}$. The time-evolution operator $e^{-i\mathbf{H}t}$ and the Fermi-Dirac distribution operator $f(\mathbf{H})$ are computed with the Chebyshev polynomial method [5]. Here we use units that $\hbar = 1$.

The density of state is obtained by the Fourier transform of the overlap between the time-evolved state $|\varphi(t)\rangle$ and the initial state $|\varphi\rangle$ as[5, 6]

$$\rho(\varepsilon) = \frac{1}{2\pi} \int_{-\infty}^{\infty} e^{i\varepsilon t} \langle \varphi | \varphi(t) \rangle \, dt. \qquad (3)$$

All along this work, we fix the temperature to $T = 300$K. We use periodic boundary conditions in the calculations for both the optical conductivity and the density of states, and the size of the system is $2400 \times 2400$ unit

cells.

### Dipole Contribution in Optical Conductivity

For the TB Hamiltonian $\mathbf{H}$, the current operator is $J = e\dot{\mathbf{R}} = ie\left[\mathbf{H},\mathbf{R}\right]$,where $\mathbf{R} = \mathbf{R}_1 + \mathbf{R}_2$ is the dipole operator and $\mathbf{R}_1 = \sum_i \mathbf{r}_i c^+_{i,\alpha} c_{i,\alpha}$ the regular term and $\mathbf{R}_2 = \sum_{i,\alpha,\beta} \langle i,\alpha|\delta\mathbf{r}|i,\beta\rangle\, c^+_{i,\alpha} c_{i,\beta}$ the inter atomic term. We have

$$\begin{aligned}
[\mathbf{H},\mathbf{R}_1] &= -\sum_{i,j,\alpha\prime,\beta\prime} t^{ij}_{\alpha\prime\beta\prime} \left(\mathbf{r}_j - \mathbf{r}_i\right) c^+_{i,\alpha\prime} c_{j,\beta\prime}, \\
[\mathbf{H},\mathbf{R}_2] &= -\sum_{i,j}\sum_{\alpha,\beta,\gamma} \Big[ t^{ij}_{\alpha\gamma} \langle\gamma|\delta\mathbf{r}|\beta\rangle \\
&\quad - t^{ij}_{\gamma\beta} \langle\alpha|\delta\mathbf{r}|\gamma\rangle \Big] c^+_{i,\alpha} c_{j,\beta} \qquad (4)
\end{aligned}$$

By neglecting the overlap from different sites, the nonzero dipole term for fluorinated graphene is given by

$$\begin{aligned}
[\mathbf{H},\mathbf{R}_2] = -\sum_{i,\alpha=p_x,p_y,p_z} &\left[\left(\varepsilon_{i,s} - \varepsilon_{i,\alpha}\right) \langle s|\delta\mathbf{r}|\alpha\rangle\, c^+_{i,s} c_{i,\alpha}\right. \\
&\left. + \left(\varepsilon_{i,\alpha} - \varepsilon_{i,s}\right) \langle\alpha|\delta\mathbf{r}|s\rangle\, c^+_{i,\alpha} c_{i,s}\right], (5)
\end{aligned}$$

where $\varepsilon_{i,\alpha}$ denotes the corresponding onsite energies and $s$ the carbon $s$ orbital.

### Complete Spectrum of the Optical Conductivity

Fig. 5 shows the complete spectrum of the in-plane and out-of-plane conductivity of fluorinated graphene with randomly distributed unpaired or paired fluorine atoms. Unlike the energy range ($\omega < 10\,\text{eV}$), shown in Fig. 1 of the main text, the optical conductivity at higher energies are highly enhanced due to the presence of fluorine adatoms. The paired and unpaired configurations are clearly distinguishable in the out-of-plane conductivity between 20 and 25 eV: two peaks centered about 21 and 22.7 eV exist for partially fluorinated graphene with paired adatoms, which are missing in the unpaired case.

## EFFECT OF RANDOMNESS AND SAMPLE SIZE

The accuracy of our numerical methods in the TB calculation of optical conductivity and density of states is mainly controlled by the sample size, and a larger sample leads to better results (see more details in Ref. 5 and 6). For a system as large as the one used in our simulations ($2400 \times 2400$), one random configuration of disordered system includes different kinds of local structures, therefore it is not necessary to average the results from different random configurations, or use even larger sample. That is, the numerical results are no longer sensitive to the randomness of the structure or the sample size. For example, as the results shown in Fig. 6, we consider partially fluorinated graphene with fixed concentration of fluorine atoms, but change the configuration of occupied sites according to different random sequences, or use larger sample size ($3600 \times 3600$). In each case the randomly occupied sites are totally different, but the numerical results are consistent. This is a direct proof that our result is not only valid for a particular "random" configuration but valid in general. It contains an average from different kinds of local structures, and does not depend on the choice of random sequence if the system size is large enough.

## REAL SPACE DISTRIBUTION OF MIDGAP STATES

For disordered partially and fully fluorinated graphene without carbon vacancies, the calculation of quasi-eigenstates shows that the dominating orbitals in the midgap states are carbon $p_z$ orbitals. The quasi-eigenstate $|\Phi(E)\rangle$, which is a superposition of the degenerate eigenstates with the same eigenenergy $E$, is obtained as the Fourier transform of $|\varphi(t)\rangle$, i.e. $|\Phi(E)\rangle = \frac{1}{2\pi}\int_{-\infty}^{\infty} dt e^{iEt} |\varphi(t)\rangle$ . The quasi-eigenstate is not exactly an energy eigenstate, but rather an approximation to it[5]. However one can still use the real space distribution of the amplitude to examine the localization of the modes [5]. In Fig. 7, we show the impurity states in real space. Probability distributions projected onto the carbon $p_z$ orbitals are shown for midgap states in partially fluorinated graphene with different types of structural disorder. The results indicate that the midgap states are all quasilocalized around the unfluorinated carbon atoms near the fluorinated sites, except for the cases with paired fluorine atoms.

For fully fluorinated graphene with carbon vacancies, the dominating orbitals of the midgap states around the energy peak at $E = 0.9$ eV are carbon $p_x$ and $p_y$ orbitals (see the orbital components in the left panel of Fig. 8), quasilocalized around the vacancies (see the real space distribution of carbon $p_y$ orbital in the right panel of Fig. 8).

* s.yuan@science.ru.nl

[1] Actually simple DFT calculations would describe the graphene band structure accurate. But to handle both parts of the model on the same footing we used the $G_0W_0$ method for graphene as well.

[2] G. Kresse and J. Hafner, J. Phys.: Condens. Matter **6**, 8245 (1994).

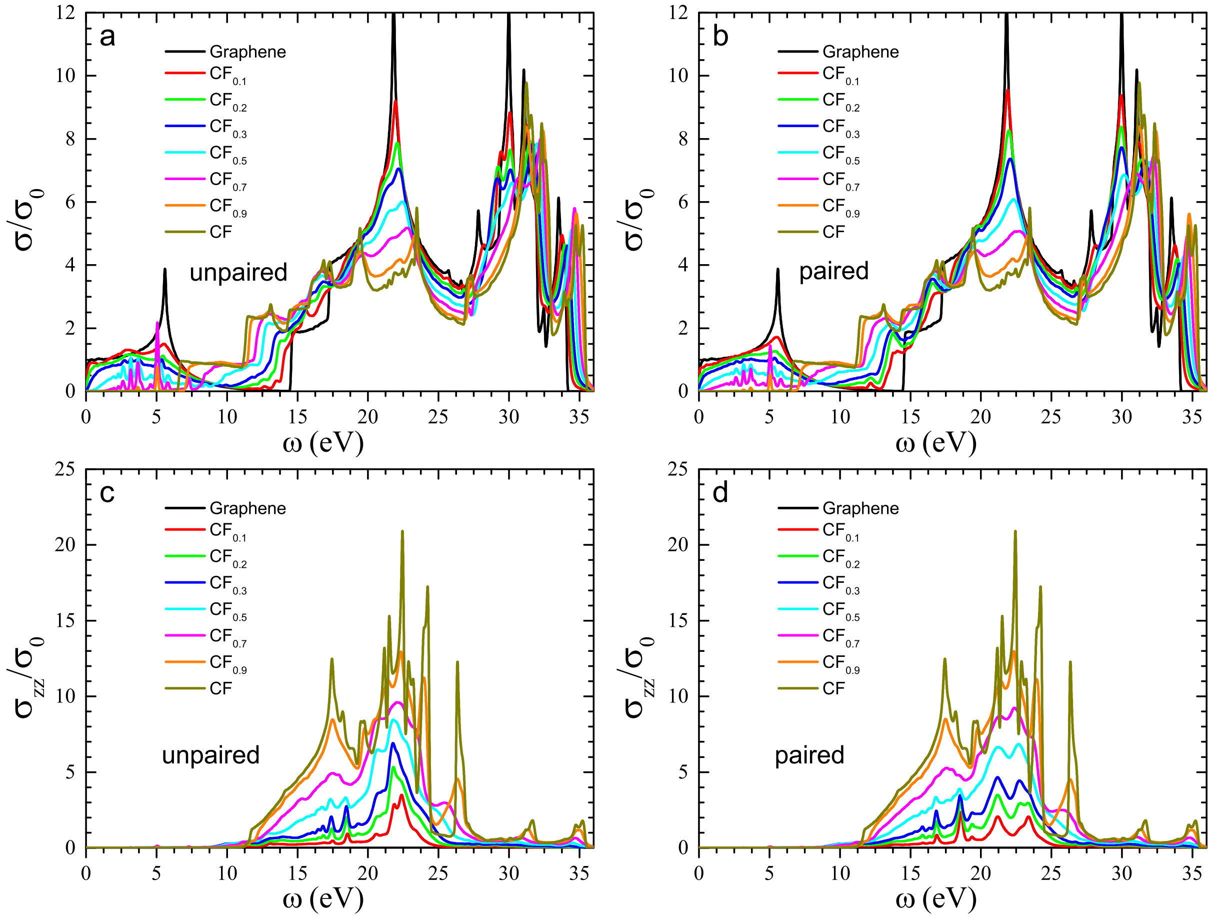


Figure 5. (a,b) In-plane and (c,d) out-of-plane optical conductivity of partially and fully fluorinated graphene with different concentration of randomly distributed unpaired (left panels) or paired (right panels) fluorine adatoms.

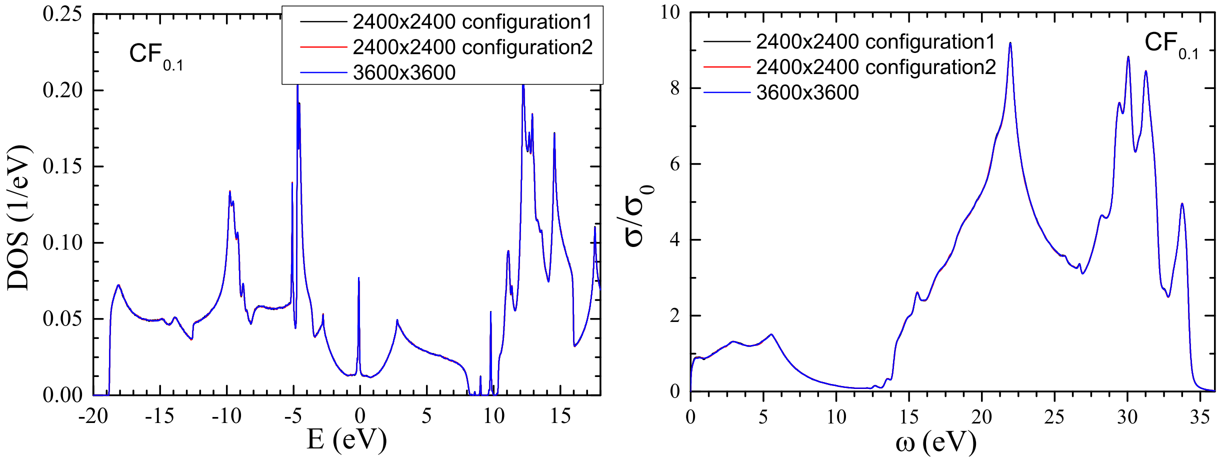


Figure 6. DOS and optical spectrum of partially fluorinated graphene ($CF_0.1$) with different configuration of random distributed fluorine atoms, or with different sample size.

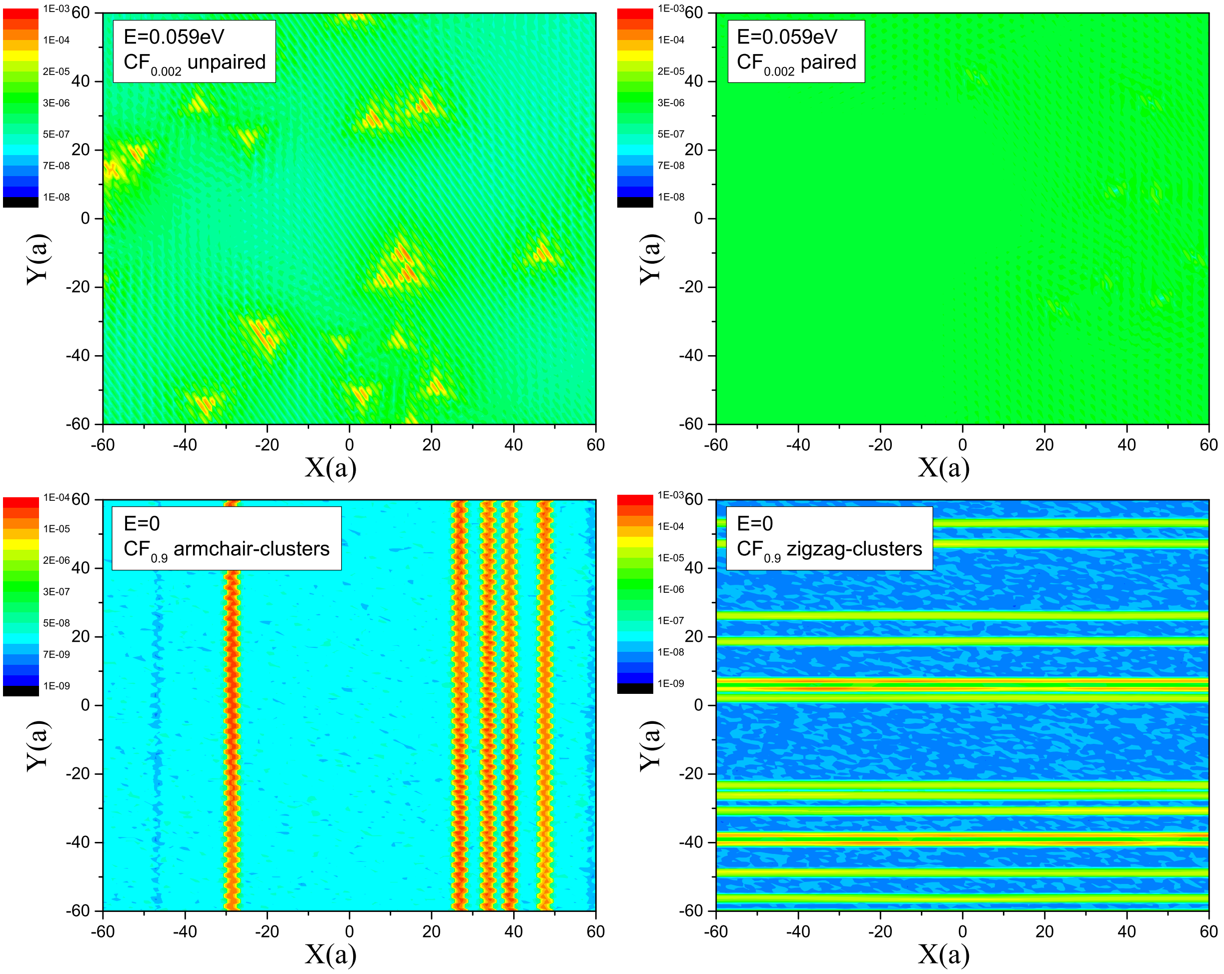


Figure 7. Real space distribution of carbon $P_z$ orbital of midgap states for partially fluorinated graphene, with different types of structure disorder.

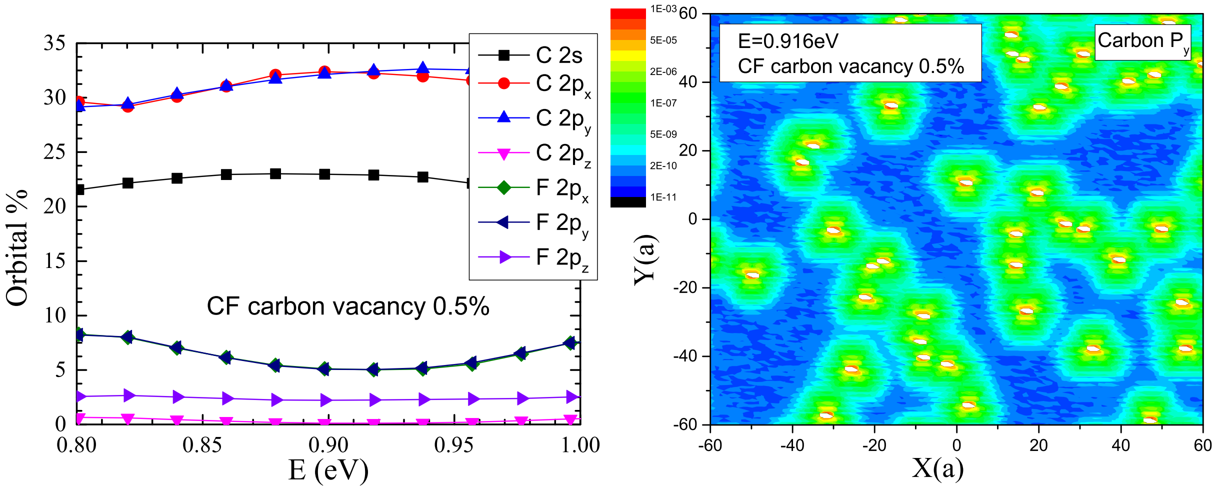


Figure 8. Orbital components (left) and real space distribution of carbon $P_y$ orbital (right) of midgap states for fully fluorinated graphene with carbon vacancies. The white points indicate the position of the vacancies.

[3] F. Karlicky and M. Otyepka, Journal of Chemical Theory and Computation **9**, 4155 (2013).

[4] A. Ishihara, *Statistical Physics* (Academic Press, New York, 1971).

[5] S. Yuan, H. De Raedt, and M. I. Katsnelson, Phys. Rev. B **82**, 115448 (2010).

[6] A. Hams and H. De Raedt, Phys. Rev. E **62**, 4365 (2000).
